# Supplementary material for: Bit-by-Bit: Progressive QAT Strategy with Outlier Channel Splitting for Stable Low-Bit LLMs
Source: arXiv:2604.07888 source file (2026-04-09)
Supplement: Supplementary file 1 [file appendix_CMTQ.tex]

\begin{algorithmic}[1]
\Function{ProgressiveQuantize}
    \textbf{Phase 1: Coarse-to-fine quantization from 8-bit down to $(k+2)$-bit}
    \For{$n = 8$ \textbf{to} $k+2$}
        \For{$t = 1$ \textbf{to} $T_s$}
            \State $\mathcal{L} \gets \mathcal{L}_{\text{qn}}(\mathbf{W}, n)$
            \State $\mathbf{W} \gets \mathbf{W} + \gamma \cdot \nabla_{\mathbf{W}} \mathcal{L}$ \textbf{STE in backward pass}
        \EndFor
    \EndFor

    \textbf{Phase 2: Cyclic refinement between $(k+1)$-bit and $k$-bit}
    \For{$c = 1$ \textbf{to} $C$}
        \For{$t = 1$ \textbf{to} $T_c$}
            \State $\mathcal{L} \gets \mathcal{L}_{\text{qn}}(\mathbf{W}, k+1)$
            \State $\mathbf{W} \gets \mathbf{W} + \gamma \cdot \nabla_{\mathbf{W}} \mathcal{L}$
        \EndFor
        \For{$t = 1$ \textbf{to} $T_c$}
            \State $\mathcal{L} \gets \mathcal{L}_{\text{qn}}(\mathbf{W}, k)$
            \State $\mathbf{W} \gets \mathbf{W} + \gamma \cdot \nabla_{\mathbf{W}} \mathcal{L}$
        \EndFor
    \EndFor

    \textbf{Phase 3: Final fine-tuning at $k$-bit}
    \For{$t = 1$ \textbf{to} $T_f$}
        \State $\mathcal{L} \gets \mathcal{L}_{\text{qn}}(\mathbf{W}, k)$
        \State $\mathbf{W} \gets \mathbf{W} + \gamma \cdot \nabla_{\mathbf{W}} \mathcal{L}$
    \EndFor

    \State \Return $\mathbf{W}$
\EndFunction
\end{algorithmic}
