# Supplementary material for: Bit-by-Bit: Progressive QAT Strategy with Outlier Channel Splitting for Stable Low-Bit LLMs
Source: arXiv:2604.07888 source file (2026-04-09)
Supplement: Supplementary file 2 [file appendix-table1.tex]

% ------------------ 表格开始 ------------------
\begin{table}[htbp]
    \centering
    \caption{EfficientQAT of Llama-3 series in groupsize = 128}
    \label{tab:efficientqat_group128}
    
    % 使用 \resizebox 强制表格宽度为 \textwidth (文本宽度)，解决表格超宽问题
    \resizebox{\textwidth}{!}{
    \small 
    \begin{tabular}{@{}lll rrrrrr@{}}
        \toprule
        \textbf{Model Size} & \textbf{Configuration} & \textbf{Setting} & \textbf{PIQA} & \textbf{ARC\_e} & \textbf{ARC\_c} & \textbf{Hella} & \textbf{Wino} & \textbf{task\_avg} \\
        \midrule
        
        % Llama3.2-1B Group
        \multirow{\textbf{Llama3.2-1B}} 
        & FP16 & --- & 74.54 & 60.44 & 36.01 & 63.54 & 60.70 & 59.06 \\
        \cline{2-9}
        & \underline{EfficientQAT-blockap} & w2a16, redpajama & 63.82 & 45.62 & 25.94 & 38.37 & 52.96 & 45.34 \\
        \cline{2-9}
        & EfficientQAT-blockap+e2e & w2a16, alpaca & 65.89 & 48.06 & 26.79 & 43.18 & 52.01 & 47.18 \\
        \midrule
        
        % Llama3-8B Group
        \multirow{\textbf{Llama3-8B}}
        & FP16 & --- & 80.63 & 77.82 & 53.24 & 78.06 & 72.45 & 72.64\\
        \cline{2-9}
        & \underline{EfficientQAT-blockap} & w2a2, redpajama & 54.41 & 30.35 & 22.53 & 26.54 & 50.43 & 45.34 \\
        \cline{2-9}
        & EfficientQAT-blockap+e2e & w2a2, alpaca & 57.24 & 35.19 & 23.55 & 28.95 & 51.78 & 47.18 \\
        \bottomrule
    \end{tabular}
    } % \resizebox 结束
\end{table}
% ------------------ 表格结束 ------------------
