# Supplementary material for: Bit-by-Bit: Progressive QAT Strategy with Outlier Channel Splitting for Stable Low-Bit LLMs
Source: arXiv:2604.07888 source file (2026-04-09)
Supplement: Supplementary file 3 [file appendix-table2.tex]

\begin{table}[htbp]
\centering
\caption{EfficientQAT of Llama-3 series in groupsize = 128}
\label{tab:efficientqat_group128}
\begin{tabularx}{\textwidth}{lll *{7}{Y}} % 3列 + 7个任务列
\toprule
\textbf{Model Size} & \textbf{Configuration} & \textbf{Setting} & \textbf{PIQA} & \textbf{ARC\_e} & \textbf{ARC\_c} & \textbf{Hella} & \textbf{Wino} & \textbf{task\_avg} \\
\midrule

\multirow{3}{*}{\textbf{Llama3.2-1B}} 
& FP16 & --- & 74.54 & 60.44 & 36.01 & 63.54 & 60.70 & 59.06 \\
& \underline{EfficientQAT-blockap} & w2a16 group128, redpajama & 63.82 & 45.62 & 25.94 & 38.37 & 52.96 & 45.342 \\
& EfficientQAT-blockap+e2e & w2a16 group128, alpaca & 65.89 & 48.06 & 26.79 & 43.18 & 52.01 & 47.186 \\
\midrule

\multirow{2}{*}{\textbf{Llama3-8B}} 
& \underline{EfficientQAT-blockap} & w2a2 group128, redpajama & 54.41 & 30.35 & 22.53 & 26.54 & 50.43 & 45.342 \\
& EfficientQAT-blockap+e2e & w2a2 group128, alpaca & 57.24 & 35.19 & 23.55 & 28.95 & 51.78 & 47.186 \\
\bottomrule
\end{tabularx}
\end{table}
